# Supplementary material for: Kullback-Leibler divergence between quantum distributions, and its upper-bound
Source: arXiv:2008.05932 source file (2020-12-10)
Supplement: Supplementary file 1 [file supplmat.pdf]

# Supplementary Material to Kullback–Leibler divergence between quantum distributions, and its upper-bound

Vincenzo Bonnici[1]

[1] Department of Computer Science, University of Verona, Italy

## 1 Overview

This document contains the supplementary material to the main article *Kullback-Leibler divergence between quantum distributions, and its upper-bound.*

Section 2 shows the general proof that given a quantum distribution $P$, the distribution $U_P$ maximizes the entropic divergence w.r.t. the distribution $Q$ which assigns a quantity of $M-n-1$ to the $n$-th cell, and a quantity of 1 to the $(n-1)$-th cell, in addition to the minimum quantity of 1 to each cell. the section also reports some implications that arise from the proof.

Section 3 reports additional results regarding the comparisons among the measures that are taken into account in the main article

Section 4 reports additional results regarding the relation between the measures and the properties of diverging distributions.

Section 5 reports additional results regarding differences in ranking outcomes.

## 2 Special case 1: general proof

**Proposition 2.1.** *Let $P$ to be a OQD obtained by distribution a quantity $M$ to $n$ cells. Let $U$ to be a QD which assigns all the free quantity $M-n$ to the $n$-th cell, in addition to the minimum quantity of 1 to each cell. Let $Q$ to be a QD which assigns a quantity $M-n-1$ to the $n$-th cell, and a quantity of 1 to the $(n-1)$-th cell, in addition to the minimum quantity of 1 to each cell. Then, $KL(P||U) > KL(P||Q)$.*

*Proof.* A first consideration is that from position 1 to $n-2=3$, the two divergences have identical contributions, thus they can be ignored in the comparison. Therefore, it has to be proven that:

$$P_{n-1}log_2\frac{P_{n-1}}{U_{n-1}} + P_nlog_2\frac{P_n}{U_n} > P_{n-1}log_2\frac{P_{n-1}}{Q_{n-1}} + P_nlog_2\frac{P_n}{Q_n} \tag{1}$$

.

By construction, $U_n = \frac{M-n+1}{M}$ and $U_{n-1} = \frac{1}{M}$, while $Q_n = \frac{M-n}{M}$ and $Q_{n-1} = \frac{2}{M}$. Thus Equation 1 can be written as:

$$P_{n-1}log_2\frac{P_{n-1}}{\frac{1}{M}} + P_nlog_2\frac{P_n}{\frac{M-n+1}{M}} > P_{n-1}log_2\frac{P_{n-1}}{\frac{2}{M}} + P_nlog_2\frac{P_n}{\frac{M-n}{M}} \quad (2)$$

, that is

$$\begin{gathered} P_{n-1}log_2P_{n-1} - P_{n-1}log_2\frac{1}{M} + P_nlog_2P_n - P_nlog_2\frac{M-n+1}{M} > \\ P_{n-1}log_2P_{n-1} - P_{n-1}log_2\frac{2}{M} + P_nlog_2P_n - P_nlog_2\frac{M-n}{M} \end{gathered} \quad (3)$$

, and therefore, by removing equal terms from the left and right sides of the inequality,

$$-P_{n-1}log_2\frac{1}{M} - P_nlog_2\frac{M-n+1}{M} > -P_{n-1}log_2\frac{2}{M} - P_nlog_2\frac{M-n}{M} \quad (4)$$

, that is

$$\begin{gathered} -P_{n-1}log_2(1) + P_{n-1}log_2(M) - P_nlog_2(M-n+1) + P_nlog_2(M) > \\ -P_{n-1}log_2(2) + P_{n-1}log_2(M) - P_nlog_2(M-n) + P_nlog_2(M) \end{gathered} \quad (5)$$

, therefore, since $log_2(1) = 0$ and by removing equal terms,

$$-P_nlog_2(M-n+1) > -P_{n-1}log_2(2) - P_nlog_2(M-n) \quad (6)$$

.

For this specific case, the difference between $P_n$ and $P_{n-1}$ is given by a single element. However, since $P$ is ordered, it can be assumed that there is a discretized gap between the two positions such that $P_{n-1} = P_n + \epsilon$, for $\epsilon \in \mathbb{N}, \geq 0$. Thus, the inequality can be written, by also changing the verse of it, as

$$P_nlog_2(M-n+1) < (P_n+\epsilon)log_2(2) + P_nlog_2(M-n) \quad (7)$$

, that is

$$P_nlog_2(M-n+1) < P_nlog_2(2) + \epsilon log_2(2) + P_nlog_2(M-n) \quad (8)$$

, that is

$$P_nlog_2(M-n+1) - P_nlog_2(2) - P_nlog_2(M-n) < \epsilon log_2(2) \quad (9)$$

, that is

$$P_n\Bigg(log_2(M-n+1) - log_2(2) - log_2(M-n)\Bigg) < \epsilon log_2(2) \quad (10)$$

.

It can be assumed that $P_n = k\epsilon$, for a given factor $k \in \mathbb{R}, > 0$, thus $P_n$ can be greater or smaller that $\epsilon$. In addition, $log_2(M-n+1) - log_2(2) - log_2(M-n)$ equals $log_2 \frac{M-n+1}{2(M-n)}$. Thus the inequality can be written as

$$k\epsilon\left(log_2 \frac{M-n+1}{2(M-n)}\right) < \epsilon log_2(2) \tag{11}$$

, and, therefore

$$k\left(log_2 \frac{M-n+1}{2(M-n)}\right) < log_2(2) \tag{12}$$

. If $M-n > 1$, which is always true because a minimum amount of 1 is assigned to each cell and the two distribution must be different, then $\frac{M-n+1}{2(M-n)}$ is always less than 1. This implies that $log_2 \frac{M-n+1}{2(M-n)}$ is always less than or equal to zero. Thus, independently from the value of $k$, that must be in any case $\geq 0$, the inequality is always satisfied.

More in general, Equation 12 can be written as:

$$k\left(log_2 \frac{M-n+1}{(1+x)(M-n+1-x)}\right) < log_2(1+x) \tag{13}$$

, because a given quantity $x+1$, that is at least 1 and at most $M-n+1$, is moved from position $n$ to position $n-1$.

In Equation 13, we can put $M-n+1 = y$ and thus, in order to assert than the result of the logarithm must be always less the 0, it has to be shown that

$$\begin{aligned} y &< (1+x)(y-x) \\ y &< y + xy - x - x^2 \\ 0 &< +xy - x - x^2 \\ 0 &< x(y-1) - x^2 \\ 0 &> x(1-y) + x^2 \end{aligned} \tag{14}$$

. The determinant is given by $(1-y)^2-4$ that is: equal to 0 for $M = n-4$, which is impossible because $M > n$; less than 0 for $M < n-4$ that is still impossible because $M > n$; greater than 0 for $M > n-4$. Thus, the determinant is always greater than 0 and the inequality is less than 0 which means that it admits two solutions $x_1$ and $x_2$ such that it is true for $x_1 < x < x_2$. The two solutions are given by $\frac{(y-1)\pm\sqrt{(1-y)^2-4}}{2}$. The determinant can also be written as $(1-y)^2-4 = (1-M+n-1)^2-4 = (M+n)^2-2^2$. For practical applications, the determinant can be approximated to $(M+n)^2$, thus the inequality is satisfied for $(M-n+M+n)/2 < x < (M-n-M-n)/2$, namely $-n < x < M$ that is always true because $x \leq M-n$ by definition. □

| | | Pearson corr. |
|---|---|---|
| Normalized Kullback-Leibler | Kullback-Leibler | 0.9893 |
| Normalized Kullback-Leibler | Jensen-Shannon divergence | 0.9888 |
| Normalized Kullback-Leibler | Generalized Jaccard distance | 0.9549 |
| Normalized Kullback-Leibler | Hellinger distance | 0.9881 |
| Kullback-Leibler | Jensen-Shannon divergence | 0.9926 |
| Kullback-Leibler | Generalized Jaccard distance | 0.9232 |
| Kullback-Leibler | Hellinger distance | 0.9932 |
| Jensen-Shannon divergence | Generalized Jaccard distance | 0.9441 |
| Jensen-Shannon divergence | Hellinger distance | 0.9999 |
| Hellinger distance | Generalized Jaccard distance | 0.9411 |

Table 1: Pearson's correlation among the investigated measures on two-by-two comparisons of ordered distributions generated by distributing a quantity of 15 to 5 cells.

The fact that Equation 13 is always verified implies that, independently of how the quantity is arranged in the last two positions, the distribution $U$ is the one that maximizes the entropic divergence. Besides, it also implies two other assertions. The first assertion is that if the number of cells is equal to 2 then $U$ is always the maximizing distribution. The second assertion is that if the quantity is moved from the last cell to a specific other cell, not necessary the second-last, the $U$ is still the maximizing distribution. In fact, the inequality is independent from the specific cell position and it only requires that $P_i = P_n + \epsilon$ and that $P_n = k\epsilon$, thus $P_i = k\epsilon + \epsilon = \epsilon(k+1)$ which means that $P_i$ must be greater than $P_n$. This consideration highlights the fact that $U$ is the distribution that assigns all the available quantity to the cell having the smallest probability in $P$, thus it is independent of the ordering.

# 3 Comparisons between measures

Table 1 reports the Pearson's correlation among the five measures that are compared in the main article. Correlations are calculated by taking into account the values of the measures in computing the divergence (dissimilarity) between ordered distributions. The distributions are built by distributing a quantity of 15 to 5 cells.

# 4 Correlation with distributional properties

Table 2 reports Pearson correlation coefficients among the investigated measures on comparing ordered distributions with the uniform one generated by distributing a quantity of 32 to 8 cells.

Figure 1 shows the relation of the compared measures with the Kurtosis's index, and Figure 2 shows the relation with the skewness. It has to be noticed that some values of the skewness and Kurtosis statistics may appear unexpected, however, such an unexpected behaviour is because relatively small (in their cardinality) distributions are taken into account. Besides, the generate distributions are more similar to exponential distributions rather than normal ones. For

| | | Pearson |
|---|---|---|
| Normalized Kullback-Leibler | Entropy | -0.9892 |
| Kullback-Leibler | Entropy | -0.9999 |
| Jensen-Shannon divergence | Entropy | -0.9804 |
| Generalized Jaccard distance | Entropy | -0.9232 |
| Hellinger distance | Entropy | -0.9932 |
| | | Pearson |
| Normalized Kullback-Leibler | Coefficient of variation | 0.9872 |
| Kullback-Leibler | Coefficient of variation | 0.9832 |
| Jensen-Shannon divergence | Coefficient of variation | 0.9678 |
| Generalized Jaccard distance | Coefficient of variation | 0.9181 |
| Hellinger distance | Coefficient of variation | 0.9649 |
| | | Pearson |
| Normalized Kullback-Leibler | Skewness | 0.6343 |
| Kullback-Leibler | Skewness | 0.6096 |
| Jensen-Shannon divergence | Skewness | 0.6554 |
| Generalized Jaccard distance | Skewness | 0.5143 |
| Hellinger distance | Skewness | 0.5475 |
| | | Pearson |
| Normalized Kullback-Leibler | Kurtosis | 0.4715 |
| Kullback-Leibler | Kurtosis | 0.4795 |
| Jensen-Shannon divergence | Kurtosis | 0.5170 |
| Generalized Jaccard distance | Kurtosis | 0.2622 |
| Hellinger distance | Kurtosis | 0.3995 |

Table 2: Pearson correlation coefficients among the investigated measures on comparing ordered distributions with the uniform one generated by distributing a quantity of 32 to 8 cells.

example, only positive values of skewness are expected because the examined distributions are monotonically ordered, however, the distribution which values are $(7, 7, 7, 7, 1, 1, 1, 1)$ has a skewness of 0 because mean, mode and median of the distribution have the same value. The distribution $(7, 7, 6, 6, 3, 1, 1, 1)$ has a negative skewness because the mode (1) smaller than the mean (4).

## 5 Differences in ranking outcomes

Table 3 show the Spearman rank correlations among the investigated measures on comparing ordered distributions with the uniform one generated by distributing a quantity of 32 to 8 cells.

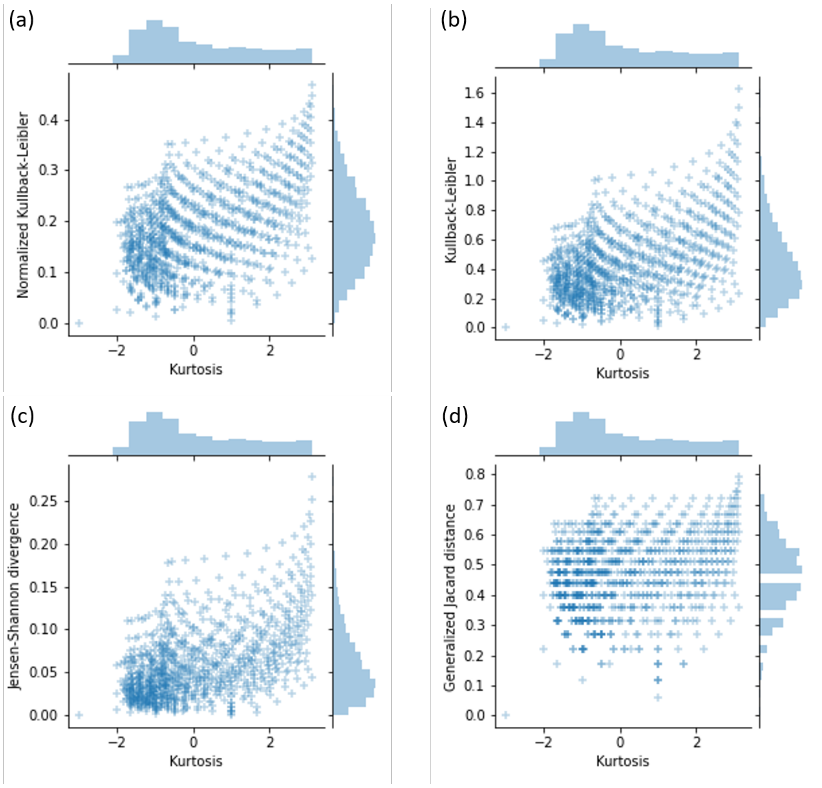


Figure 1: Scatter plots generated by putting in relation four of the investigated measures and the Kurtosis index of the set of monotonically ordered distributions, generated with 8 cells and 32 dots, and the corresponding uniform distribution.

| | | Spearman |
|---|---|---|
| Normalized Kullback-Leibler | Kullback-Leibler | 0.9989 |
| Normalized Kullback-Leibler | Jensen-Shannon divergence | 0.9909 |
| Normalized Kullback-Leibler | Generalized Jaccard distance | 0.9695 |
| Normalized Kullback-Leibler | Hellinger distance | 0.9905 |
| Kullback-Leibler | Jensen-Shannon divergence | 0.9947 |
| Kullback-Leibler | Generalized Jaccard distance | 0.9695 |
| Kullback-Leibler | Hellinger distance | 0.9946 |
| Jensen-Shannon divergence | Generalized Jaccard distance | 0.9742 |
| Jensen-Shannon divergence | Hellinger distance | 1.0000 |
| Hellinger distance | Generalized Jaccard distance | 0.9728 |

Table 3: Spearman rank correlations among the investigated measures on comparing ordered distributions with the uniform one generated by distributing a quantity of 32 to 8 cells.

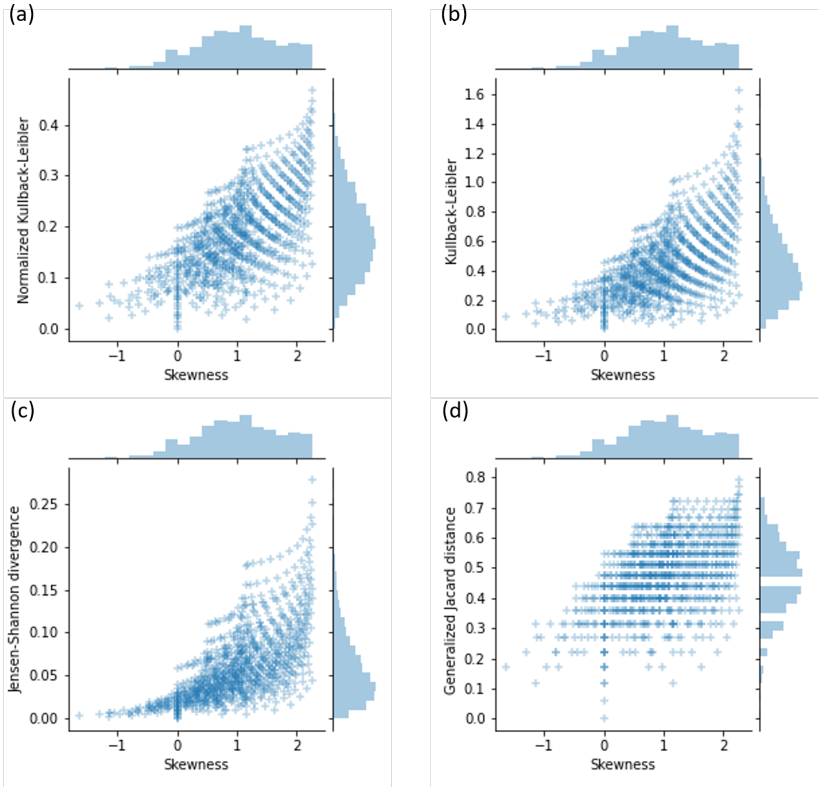


Figure 2: Scatter plots generated by putting in relation four of the investigated measures and the skewness of the set of monotonically ordered distributions, generated with 8 cells and 32 dots, and the corresponding uniform distribution.
